# Supplementary material for: Freestanding {\chi}_3-Borophene Nanoribbons: A Density Functional Theory Investigation
Source: arXiv:1712.07220 source file (2018-04-11)
Supplement: Supplementary file 1 [file sM.pdf]

## *Electronic Supplementary Material*

# *Freestanding $\chi_3$-Borophene Nanoribbons: A Density Functional Theory Investigation*

*Sahar Izadi Vishkayi, and Meysam Bagheri Tagani*

Department of Physics, Computational Nanophysics Laboratory (CNL), University of Guilan, Po Box:41335-1914, Rasht, Iran.

Fig. S1: (a) The electron density, (b) the electron localized function with isovalue equal to 0.9, (c) the transmission pathway (at zero energy, and threshold of transmission pathway's weight is equal to 0.2. The scoral bar for the weight of transmission pathway's arrows is shown in Fig.3) of *12XBNR*. (the dashed rectangle shows the unit cell of the ribbon).

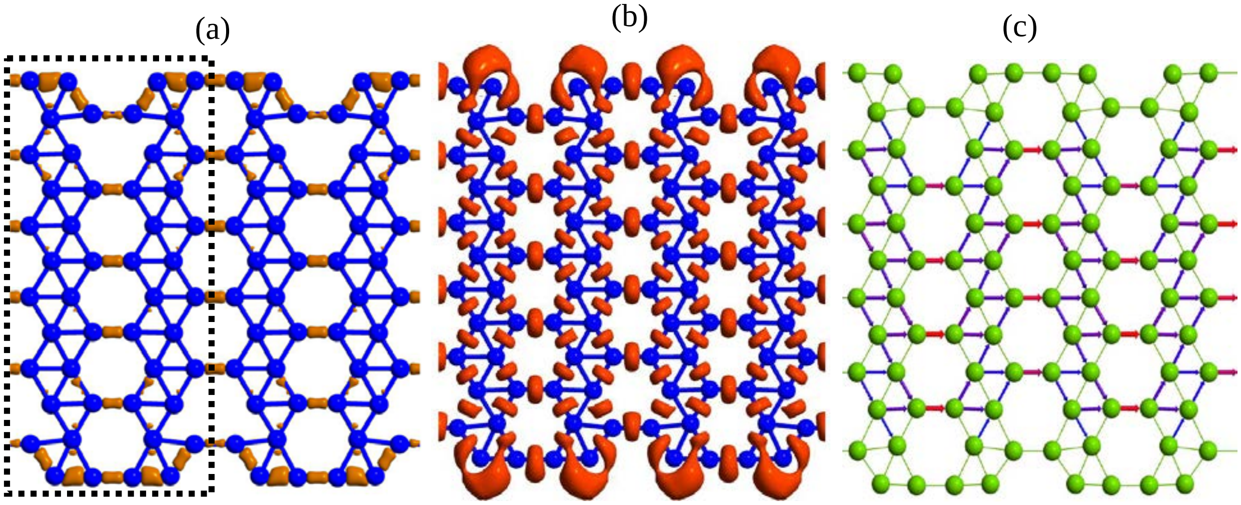


*Fig. S1*

Fig. S2: (a), (b) and (c) left to right: the electron density, the spin density, the transmission pathway of spin-up electrons, the transmission pathway of spin-down electrons, and the transmission coefficients versus energy of *26aaYBNR* in FM configuration, AFM configuration, and *26bdYBNR*, respectively. (d) left to right: the electron density, the electron localized function, the transmission pathway of electrons, and the transmission coefficient of *26ccYBNR*. The parameters are similar to the ones in Fig.4.

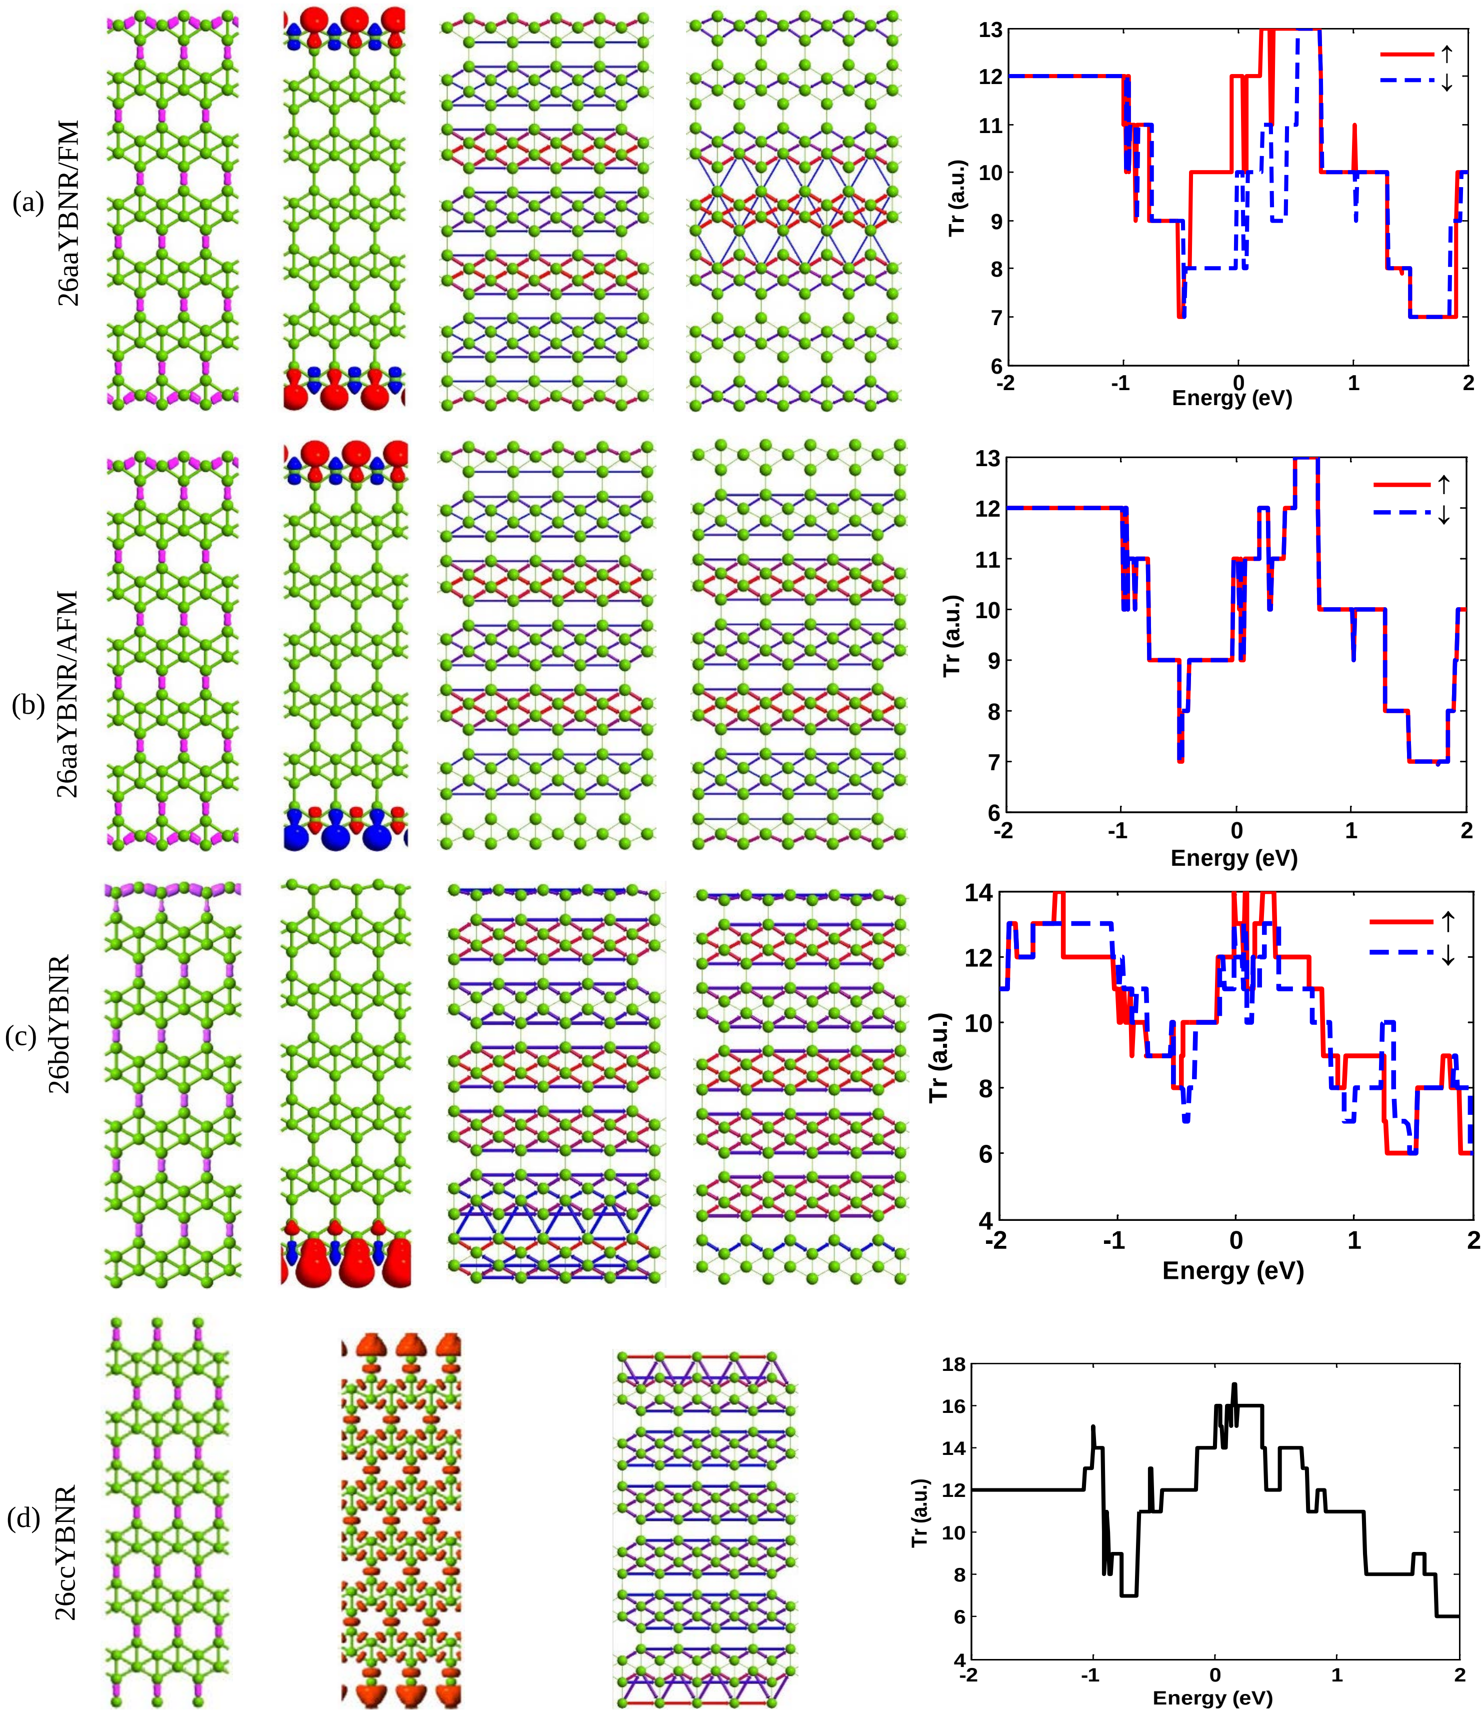
(a)
26aaYBNR/FM
(b)
26aaYBNR/AFM
(c)
26bdYBNR
(d)
26ccYBNR
Tr (a.u.)
Energy (eV)
↑
↓

*Fig. S2*

Fig. S3: (a) and (b) Left to right: the electron density, the spin density, the transmission pathway of spin-up electrons, the transmission pathway of spin-down electrons, and the transmission coefficients versus energy of *27abYBNR* in FM configuration and AFM configuration, respectively. (c) Left to right: the electron density, the electron localized function, the transmission pathway of electrons, and the transmission coefficient of *27cdYBNR*. The parameters are similar to the ones in Fig.4.

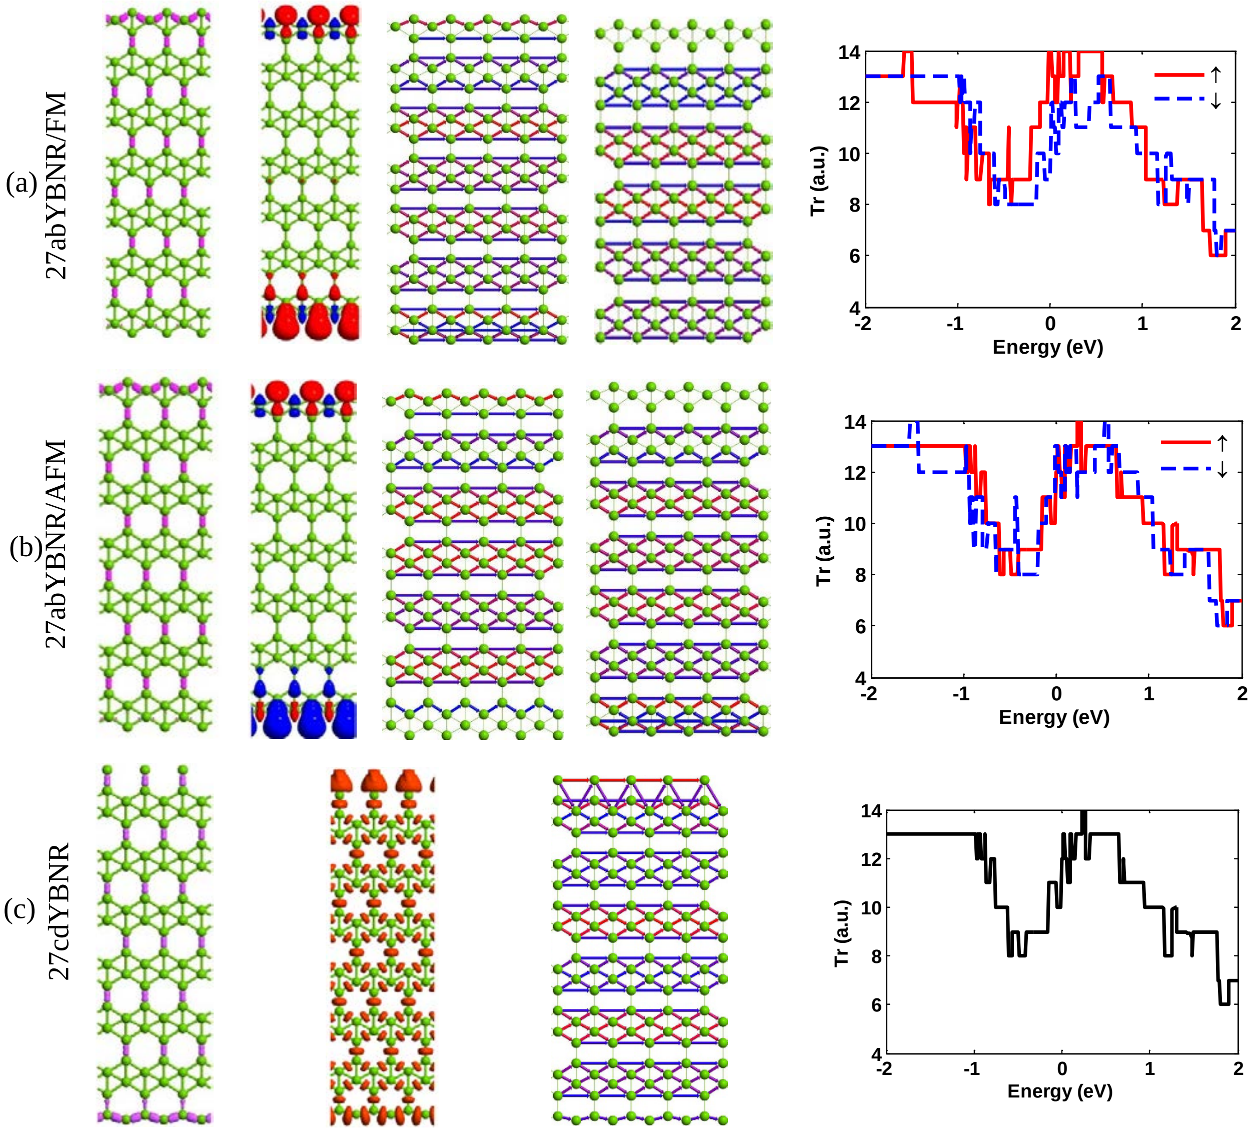


*Fig. S3*

Fig. S4: (a), (b) and (c) Left to right: the electron density, the spin density, the transmission pathway of spin-up electrons, the transmission pathway of spin-down electrons, and the transmission coefficients versus energy of *28bbYBNR* in FM configuration, AFM configuration, and *28acYBNR*. (d) Left to right: the electron density, the electron localized function, the transmission pathway of electrons, and the transmission coefficient of *28ddYBNR*. The parameters are similar to the ones in Fig.4.

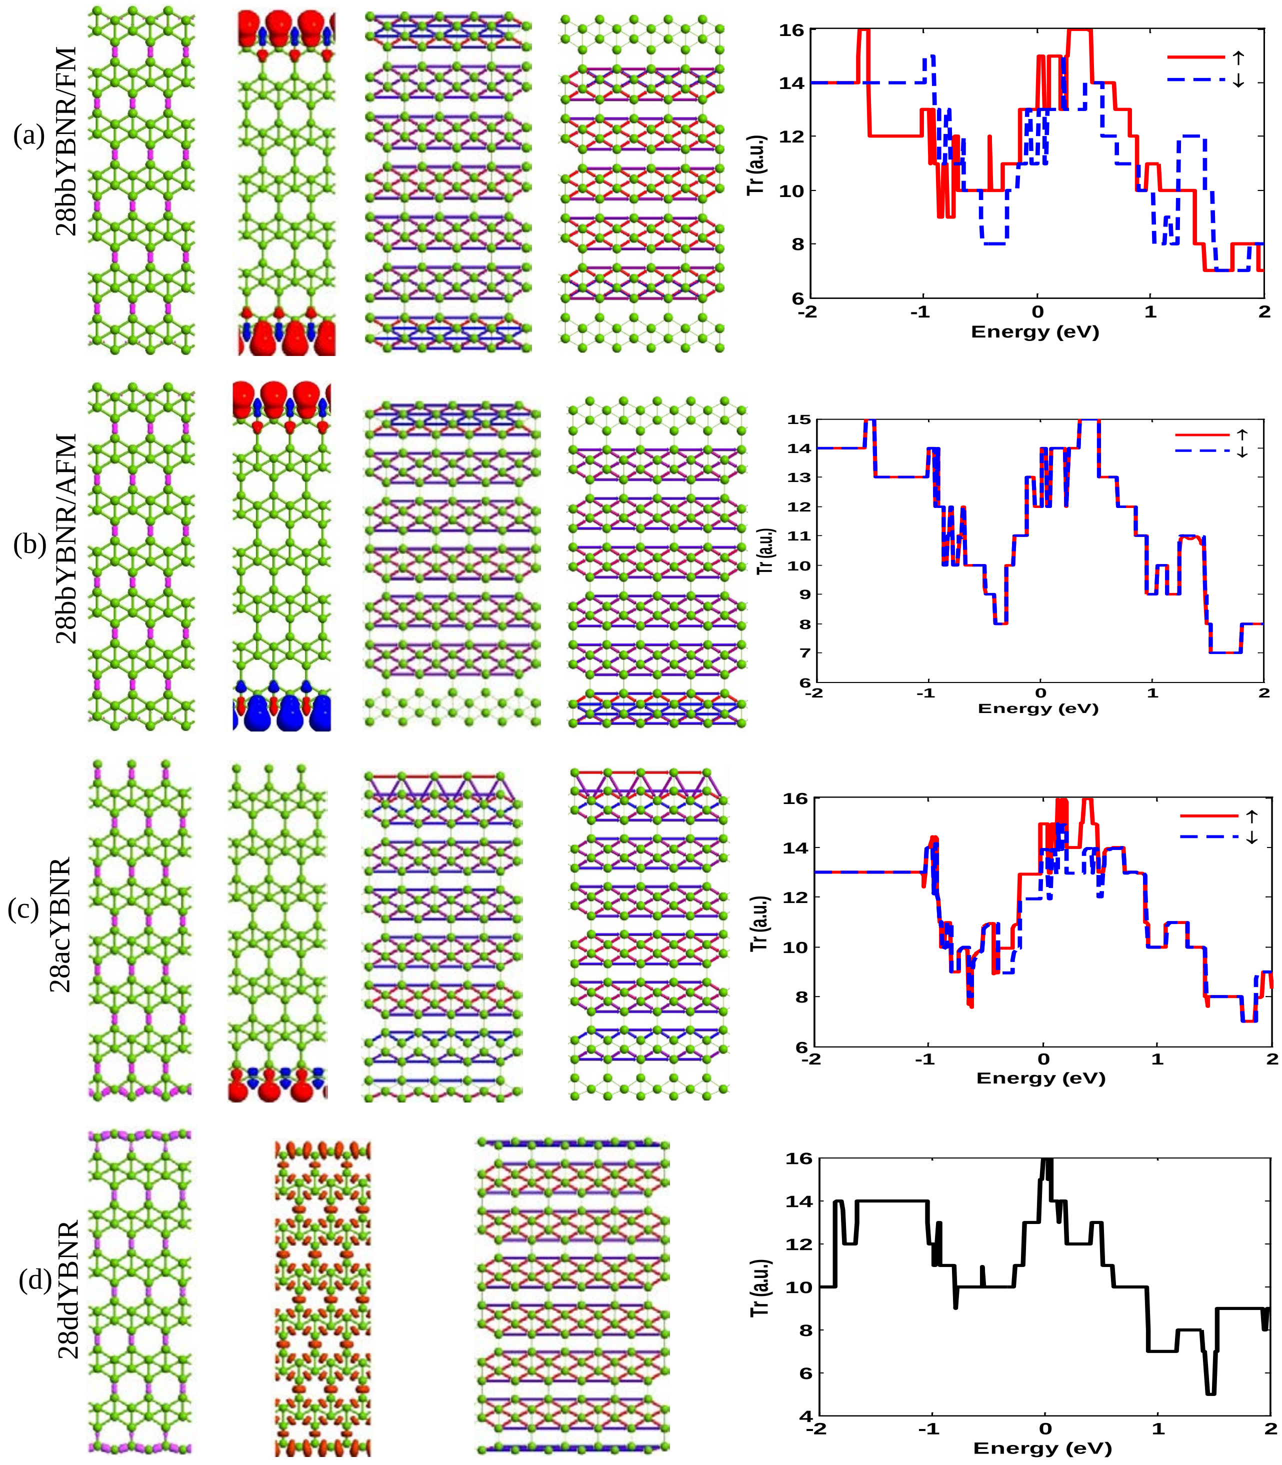


*Fig. S4*

Fig. S5: Ab-initio molecular dynamic, calculated by density functional tight binding (DFTB) approach for (a) 12XBNR, (b) 13XBNR, (c) 26aaYBNR and (d) 26ccYBNR after 2ps at room temperature.

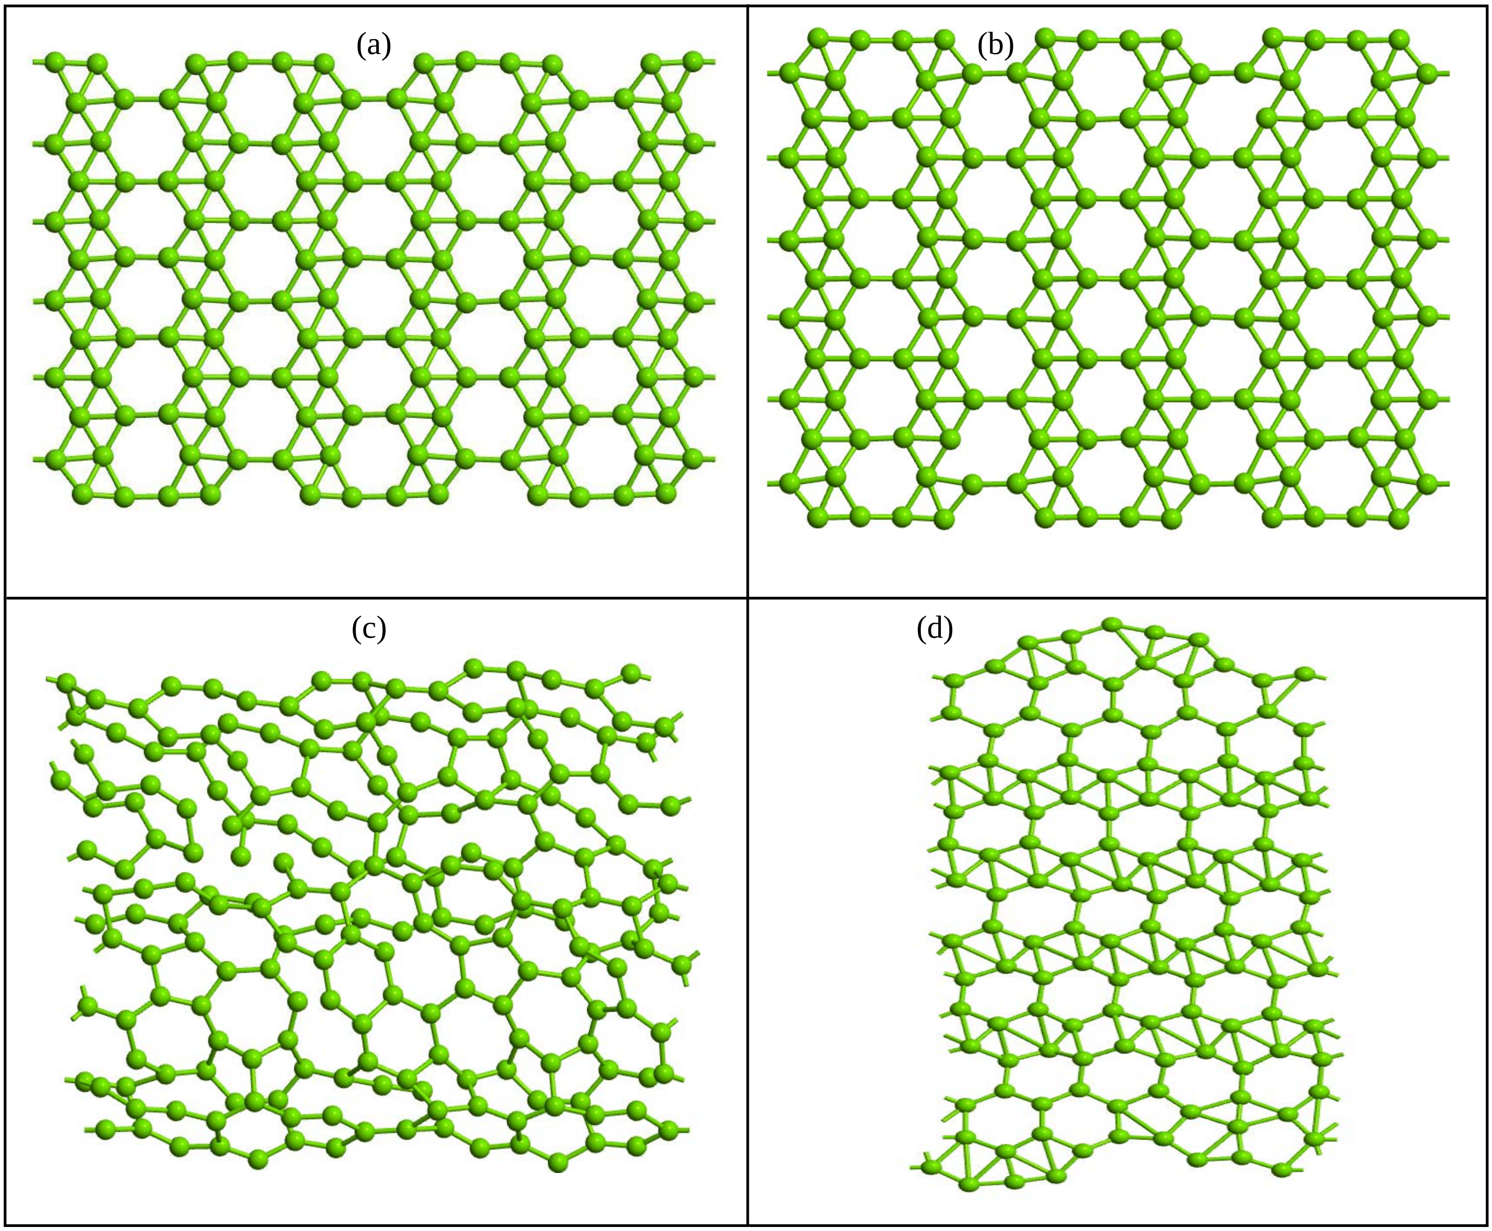


*Fig. S5*

Table S1: The bonding lengths of edge atoms of investigated *YBNRs*.

| *YBNR* | 1st Edge | | | | | | | 2nd Edge | | | | | | |
|---|---|---|---|---|---|---|---|---|---|---|---|---|---|---|
| | 1-2 | 1-3 | 2-3 | 2-4 | 3-4 | 3-5 | 4-5 | 1-2 | 1-3 | 2-3 | 2-4 | 3-4 | 3-5 | 4-5 |
| *21ad* | 1.619 | 1.633 | 1.798 | * | * | * | * | 1.529 | 2.484 | 1.650 | 3.002 | 1.771 | * | * |
| *25ad* | 1.615 | 1.634 | 1.796 | * | * | * | * | 1.527 | 2.493 | 1.653 | 3.002 | 1.767 | * | * |
| *29ad* | 1.616 | 1.634 | 1.794 | * | * | * | * | 1.527 | 2.450 | 1.651 | 3.000 | 1.767 | * | * |
| *21bc* | 1.683 | 1.685 | 1.705 | 1.797 | 1.741 | * | * | 1.654 | 2.921 | 1.708 | 1.706 | 1.691 | 1.746 | 1.729 |
| *25bc* | 1.683 | 1.685 | 1.706 | 1.800 | 1.741 | * | * | 1.652 | 2.921 | 1.709 | 1.708 | 1.691 | 1.746 | 1.729 |
| *29bc* | 1.684 | 1.684 | 1.708 | 1.798 | 1.742 | * | * | 1.653 | 2.920 | 1.710 | 1.706 | 1.693 | 1.746 | 1.731 |
| *22aa* | 1.606 | 1.639 | 1.781 | * | * | * | * | 1.606 | 1.639 | 1.781 | * | * | * | * |
| *26aa* | 1.607 | 1.638 | 1.781 | * | * | * | * | 1.607 | 1.638 | 1.781 | * | * | * | * |
| *30aa* | 1.607 | 1.638 | 1.782 | * | * | * | * | 1.607 | 1.638 | 1.782 | * | * | * | * |
| *22bd* | 1.695 | 1.681 | 1.724 | 1.794 | 1.751 | * | * | 1.528 | 2.493 | 1.654 | 3.002 | 1.768 | * | * |
| *26bd* | 1.694 | 1.680 | 1.723 | 1.792 | 1.751 | * | * | 1.527 | 2.490 | 1.652 | 3.001 | 1.768 | * | * |
| *30bd* | 1.693 | 1.681 | 1.722 | 1.793 | 1.750 | * | * | 1.526 | 2.492 | 1.652 | 3.000 | 1.766 | * | * |
| *22cc* | 1.652 | 2.922 | 1.707 | 1.709 | 1.686 | 1.746 | 1.726 | 1.652 | 2.922 | 1.707 | 1.709 | 1.686 | 1.746 | 1.726 |
| *26cc* | 1.654 | 2.921 | 1.708 | 1.706 | 1.690 | 1.747 | 1.729 | 1.654 | 2.921 | 1.708 | 1.706 | 1.690 | 1.747 | 1.729 |
| *30cc* | 1.653 | 2.921 | 1.709 | 1.707 | 1.690 | 1.746 | 1.729 | 1.653 | 2.921 | 1.709 | 1.707 | 1.690 | 1.746 | 1.729 |
| *23ab* | 1.606 | 1.638 | 1.780 | * | * | * | * | 1.685 | 1.683 | 1.709 | 1.798 | 1.743 | * | * |
| *27ab* | 1.607 | 1.638 | 1.781 | * | * | * | * | 1.686 | 1.684 | 1.710 | 1.797 | 1.743 | * | * |
| *31ab* | 1.607 | 1.638 | 1.781 | * | * | * | * | 1.685 | 1.684 | 1.710 | 1.799 | 1.744 | * | * |
| *23cd* | 1.651 | 2.918 | 1.718 | 1.703 | 1.709 | 1.743 | 1.739 | 1.527 | 2.492 | 1.652 | 3.000 | 1.767 | * | * |
| *27cd* | 1.652 | 2.918 | 1.718 | 1.703 | 1.707 | 1.743 | 1.738 | 1.526 | 2.493 | 1.652 | 3.000 | 1.765 | * | * |
| *31cd* | 1.651 | 2.918 | 1.717 | 1.704 | 1.706 | 1.744 | 1.737 | 1.525 | 2.495 | 1.652 | 3.000 | 1.764 | * | * |
| *24bb* | 1.685 | 1.684 | 1.709 | 1.798 | 1.743 | * | * | 1.685 | 1.684 | 1.709 | 1.798 | 1.743 | * | * |
| *28bb* | 1.685 | 1.684 | 1.709 | 1.799 | 1.743 | * | * | 1.685 | 1.684 | 1.709 | 1.799 | 1.743 | * | * |
| *32bb* | 1.686 | 1.683 | 1.710 | 1.797 | 1.744 | * | * | 1.686 | 1.683 | 1.710 | 1.797 | 1.744 | * | * |
| *24ac* | 1.605 | 1.639 | 1.778 | * | * | * | * | 1.654 | 2.921 | 1.710 | 1.706 | 1.692 | 1.746 | 1.730 |
| *28ac* | 1.605 | 1.639 | 1.778 | * | * | * | * | 1.652 | 2.920 | 1.710 | 1.707 | 1.693 | 1.746 | 1.730 |
| *32ac* | 1.607 | 1.638 | 1.780 | * | * | * | * | 1.653 | 2.920 | 1.711 | 1.705 | 1.694 | 1.746 | 1.731 |
| *24dd* | 1.537 | 2.478 | 1.652 | 3.009 | 1.781 | * | * | 1.537 | 2.478 | 1.652 | 3.009 | 1.781 | * | * |
| *28dd* | 1.534 | 2.485 | 1.654 | 3.008 | 1.777 | * | * | 1.534 | 2.485 | 1.654 | 3.008 | 1.777 | * | * |
| *32dd* | 1.533 | 2.483 | 1.652 | 3.007 | 1.776 | * | * | 1.533 | 2.483 | 1.652 | 3.007 | 1.776 | * | * |
